# Supplementary material for: Modelling the control of West Nile virus using mosquito reduction methods, vaccination of equids, and human behavioral adaptation to the usage of personal protective equipment
Source: arXiv:2509.24657 source file (2026-03-17)
Supplement: Supplementary file 1 [file Supplementary.pdf]

# Supplementary File: Modeling the control of West Nile virus using mosquito reduction methods, vaccination of equids, and human behavioral adaptation to the usage of personal protective equipment

Pride Duve\*, Felix Gregor Sauer, and Renke Lühken

Bernhard Nocht Institute for Tropical Medicine, Hamburg, Germany

Table S1: Definition of variables used in our model and their initial conditions.

| Parameter | Definition                                     | Value     | Source                    |
|-----------|------------------------------------------------|-----------|---------------------------|
| $L_M$     | mosquito larvae                                | 0         | defined by the authors    |
| $S_M$     | susceptible mosquitoes                         | 500,000   | (Laperriere et al., 2011) |
| $E_M$     | exposed mosquitoes                             | 0         | (Laperriere et al., 2011) |
| $I_M$     | infectious mosquitoes                          | 100       | (Laperriere et al., 2011) |
| $S_B$     | susceptible birds                              | 110,000   | (Laperriere et al., 2011) |
| $E_B$     | exposed birds                                  | 0         | (Laperriere et al., 2011) |
| $I_B$     | infectious birds                               | 10        | (Laperriere et al., 2011) |
| $R_B$     | recovered birds                                | 0         | (Laperriere et al., 2011) |
| $D_B$     | dead birds                                     | 0         | (Laperriere et al., 2011) |
| $S_H$     | susceptible humans                             | 2,700,000 | (Laperriere et al., 2011) |
| $E_H$     | exposed humans                                 | 0         | (Laperriere et al., 2011) |
| $I_H$     | infected humans                                | 100       | (Laperriere et al., 2011) |
| $R_H$     | recovered humans                               | 0         | (Laperriere et al., 2011) |
| $D_H$     | dead humans                                    | 0         | (Laperriere et al., 2011) |
| $x$       | fraction of susceptible humans that adopt PPEs | 0         | defined by the authors    |
| $S_E$     | susceptible equids                             | 10,700    | (Laperriere et al., 2011) |
| $V_E$     | vaccinated equids                              | 5         | defined by the authors    |
| $E_E$     | exposed equids                                 | 0         | (Laperriere et al., 2011) |
| $I_E$     | infected equids                                | 10        | (Laperriere et al., 2011) |
| $R_E$     | recovered equids                               | 0         | (Laperriere et al., 2011) |
| $D_E$     | dead equids                                    | 0         | (Laperriere et al., 2011) |

## S1 Positivity of solutions and existence of a feasible region

Our model describes a biological population. Thus, it is crucial to show that the state variables describing the populations at different compartments are always non-negative for all time  $t \geq 0$ .

**Theorem 1.** *The solutions  $L_M(t), S_M(t), E_M(t), I_M(t), S_B(t), E_B(t), I_B(t), R_B(t), D_B(t),$*

\*Corresponding author: pride.duve@bnitm.de

$S_H(t), E_H(t), I_H(t), R_H(t), D_H(t), S_E(t), E_E(t), I_E(t), R_E(t), D_E(t), x(t)$  of our model are always positive for all  $t > 0$ , subject to the initial conditions

$$L_M(0) = L_{M_0}, S_M(0) = S_{M_0}, E_M(0) = E_{M_0}, I_M(0) = I_{M_0}, S_B(0) = S_{B_0}, E_B(0) = E_{B_0}, I_B(0) = I_{B_0}, R_B(0) = R_{B_0}, D_B(0) = D_{B_0}, S_H(0) = S_{H_0}, E_H(0) = E_{H_0}, I_H(0) = I_{H_0}, R_H(0) = R_{H_0}, D_H(0) = D_{H_0}, S_E(0) = S_{E_0}, E_E(0) = E_{E_0}, I_E(0) = I_{E_0}, R_E(0) = R_{E_0}, D_E(0) = D_{E_0}, x(0) = x_0.$$

*Proof.* To prove that the solutions of our model are positive, we use proof by contradiction and we show that none of the state variables will change its sign at any time  $t \geq 0$ .

Suppose the solutions are not positive for some time  $t \geq 0$ . Then there should exist a point  $\tau \in (0, t)$  where any of the variables changes its sign or hits the value zero first. Suppose  $L_M$  is the first variable to hit zero, i.e.,  $L_M(\tau) = 0$ , then for any  $t \in (0, \tau)$ ,  $L_M(t) > 0, S_M(t) > 0, E_M(t) > 0, I_M(t) > 0, N_M(t) > 0, S_B(t) > 0, E_B(t) > 0, I_B(t) > 0, R_B(t) > 0, D_B(t) > 0, S_H(t) > 0, E_H(t) > 0, I_H(t) > 0, R_H(t) > 0, D_H(t) > 0, S_E(t) > 0, V_E(t) > 0, E_E(t) > 0, I_E(t) > 0, R_E(t) > 0, D_E(t) > 0$ , while  $\frac{dL_M(\tau)}{dt} < 0$ , i.e., is decreasing in this interval. From the first equation of our system,

$$\frac{dL_M(\tau)}{dt} = [(1-u_1)b_L\delta_M N_M(\tau) - (\mu_L + u_1 + u_2)L_M(\tau)] \left[ 1 - \frac{L_M(\tau)}{K_M} \right] - b_M L_M(\tau) = (1-u_1)b_L\delta_M N_M(\tau) > 0.$$

This contradicts the assumption that  $\frac{dL_M(\tau)}{dt} < 0$ , and thus  $L_M(t)$  cannot hit the value zero first. Similarly, we can show that none of the variables can hit the value zero, implying that the solutions remain positive for all time  $t \geq 0$ .  $\square$

## S2 Equilibrium points and the control reproductive number

The model has a WNV free equilibria  $E_0$ , where

$$E_0 = [L_M, S_M, E_M, I_M, S_B, E_B, I_B, R_B, D_B, S_H, E_H, I_H, R_H, x, D_H, S_E, V_E, E_E, I_E, R_E, D_E] \\ = [L_M^0, S_M^0, 0, 0, S_B^0, 0, 0, 0, 0, S_H^0, 0, 0, 0, 0, 0, S_E^0, V_E^0, 0, 0, 0, 0].$$

Using the next generation matrix method by [van den Driessche and Watmough \(2002\)](#), we find that the reproductive number, which is an important threshold for determining conditions for the persistence or elimination of WNV. The matrix of new infections is given by  $\mathcal{F}$ , while that of transitions is given by  $\mathcal{V}$ , where

$$\mathcal{F} = \begin{bmatrix} \lambda_{BM}S_M \\ 0 \\ \lambda_{MB}S_B \\ 0 \\ (1-x)\lambda_{MH}S_H \\ 0 \\ \lambda_{ME}S_E + (1-c_E)\lambda_{ME}V_E \\ 0 \end{bmatrix}, \quad \mathcal{V} = \begin{bmatrix} (\gamma_M + \mu_M + e_3u_3)E_M \\ -\gamma_M E_M + (\mu_M + e_3u_3)I_M \\ (\gamma_B + \mu_B)E_B \\ -\gamma_B E_B + (\alpha_B + \mu_B)I_B \\ (\gamma_H + \mu_H)E_H \\ -\gamma_H E_H + (\alpha_H + \mu_H)I_H \\ (\gamma_E + \mu_E)E_E \\ -\gamma_E E_E + (\alpha_E + \mu_E)I_E \end{bmatrix}.$$

Taking partial derivatives and evaluating at the WNV free equilibrium points, we have

$$F = \begin{bmatrix} 0 & 0 & 0 & \frac{\delta_M \beta S_B^0}{K_B} & 0 & 0 & 0 & 0 \\ 0 & 0 & 0 & 0 & 0 & 0 & 0 & 0 \\ 0 & \frac{\delta_M \beta \phi_B S_B^0}{K_M} & 0 & 0 & 0 & 0 & 0 & 0 \\ 0 & 0 & 0 & 0 & 0 & 0 & 0 & 0 \\ 0 & \frac{(1-x)\delta_M \beta \phi_H S_H^0}{K_M} & 0 & 0 & 0 & 0 & 0 & 0 \\ 0 & 0 & 0 & 0 & 0 & 0 & 0 & 0 \\ 0 & \frac{\delta_M \beta \phi_E [S_E + (1-c_E)V_E]}{K_M} & 0 & 0 & 0 & 0 & 0 & 0 \\ 0 & 0 & 0 & 0 & 0 & 0 & 0 & 0 \end{bmatrix},$$

$$V = \begin{bmatrix} \gamma_M + \mu_M + e_3 u_3 & 0 & 0 & 0 & 0 & 0 & 0 & 0 \\ -\gamma_M & \mu_M + e_3 u_3 & 0 & 0 & 0 & 0 & 0 & 0 \\ 0 & 0 & \gamma_B + \mu_B & 0 & 0 & 0 & 0 & 0 \\ 0 & 0 & -\gamma_B & \alpha_B + \mu_B & 0 & 0 & 0 & 0 \\ 0 & 0 & 0 & 0 & \gamma_H + \mu_H & 0 & 0 & 0 \\ 0 & 0 & 0 & 0 & -\gamma_H & \alpha_H + \mu_H & 0 & 0 \\ 0 & 0 & 0 & 0 & 0 & 0 & \gamma_E + \mu_E & 0 \\ 0 & 0 & 0 & 0 & 0 & 0 & -\gamma_E & \alpha_E + \mu_E \end{bmatrix}.$$

The basic reproductive number is given by the spectral radius of  $FV^{-1}$ , such that we have

$$R_0 = \sqrt{\frac{\delta_M \gamma_M(T) \beta(T)}{(\gamma_M(T) + \mu_M(T) + e_3 u_3)(\mu_M(T) + e_3 u_3)} \left[ \frac{S_M^0}{K_M} \right] \times \frac{\delta_M \gamma_B \beta(T)}{(\alpha_B + \mu_B)(\gamma_B(T) + \mu_B)} \left[ \frac{S_B^0}{K_B} \right]}. \quad (S1)$$

$S_B^0 = K_B$ . To get  $S_M^0$ , we solve the first two equations of our model when there is no infection. From the first equation, we have

$$(1 - e_1 u_1) b_L \delta_M S_M - \frac{(1 - e_1 u_1) b_L \delta_M S_M L_M}{K_M} - (\mu_L + e_1 u_1 + e_2 u_2) L_M + \frac{(\mu_L + e_1 u_1 + e_2 u_2) L_M^2}{K_M} = b_M L_M, \quad (S2)$$

while from the second equation, we have

$$S_M = \frac{b_M L_M}{(\mu_M + e_3 u_3)}. \quad (S3)$$

Solving Equations (S2) and (S3) simultaneously, we have

$$\frac{(1-e_1u_1)b_L\delta_M b_M}{(\mu_M+e_3u_3)} - \frac{(1-e_1u_1)b_L\delta_M b_M L_M}{(\mu_M+e_3u_3)K_M} - (\mu_L+e_1u_1+e_2u_2)L_M + \frac{(\mu_L+e_1u_1+e_2u_2)L_M^2}{K_M} = b_M L_M. \quad (S4)$$

Solving equation (S4) yields  $L_M = 0$  or

$$L_M = K_M \left[ 1 - \frac{b_M}{(\mu_L+e_1u_1+e_2u_2)} \times \left( \frac{1}{\left[ \frac{(1-e_1u_1)b_L\delta_M}{(\mu_L+e_1u_1+e_2u_2)} \right] \times \left[ \frac{b_M}{(\mu_M+e_3u_3)} \right] - 1} \right) \right],$$

which simplifies to

$$L_M = K_M \left[ 1 - \frac{b_M}{(\mu_L+e_1u_1+e_2u_2)[R_M-1]} \right], \text{ where } R_M = \left[ \frac{(1-e_1u_1)b_L\delta_M}{(\mu_L+e_1u_1+e_2u_2)} \right] \times \left[ \frac{b_M}{(\mu_M+e_3u_3)} \right].$$

It follows that  $L_M$  is positive if and only if  $\frac{b_M}{(\mu_L+e_1u_1+e_2u_2)(R_M-1)} < 1$ , and this is possible provided  $1 < R_M < 1 + \frac{b_M}{\mu_L+e_1u_1+e_2u_2}$ . In  $R_M$ , the term  $\frac{(1-e_1u_1)b_L\delta_M}{(\mu_L+e_1u_1+e_2u_2)}$  is the probability that mosquito larvae survive the aquatic phase, while the term  $\frac{b_M}{(\mu_M+e_3u_3)}$  is the probability that adult mosquitoes survive the adult stage.  $S_M^0$  now becomes

$$S_M^0 = \frac{b_M K_M}{(\mu_M+e_3u_3)} \left[ 1 - \frac{b_M}{(\mu_L+e_1u_1+e_2u_2)[R_M-1]} \right].$$

$$S_H^0 = \frac{b_H N_H^0}{\mu_H}, S_E^0 = \frac{b_E N_E^0}{(\mu_E+\theta_E)} \times \left[ \frac{1}{1-R_E} \right] \text{ and } V_E^0 = \frac{\theta_E b_E N_E^0}{(\mu_E+\theta_E)(\mu_E+\omega_E)} \times \left[ \frac{1}{1-R_E} \right],$$

where  $R_E = \frac{\theta_E}{(\mu_E+\theta_E)} \times \frac{\omega_E}{(\mu_E+\omega_E)}$ . The term  $\frac{\theta_E}{(\mu_E+\theta_E)}$  is the fraction of susceptible equids that get vaccinated, while the term  $\frac{\omega_E}{(\mu_E+\omega_E)}$  is the fraction of vaccinated equids that lose the vaccine-induced immunity.  $S_E^0$  and  $V_E^0$  are positive whenever  $R_E < 1$ , and this is the case since the terms  $\frac{\theta_E}{(\mu_E+\theta_E)} \times \frac{\omega_E}{(\mu_E+\omega_E)} < 1$  for all time.

**Theorem 2.** Given the optimal control variables  $(u_1^*, u_2^*, u_3^*)$  and the objective functional:

$$\begin{aligned} J &= \int_0^{T_F} A_1 L_M + A_2 N_M + A_3 (E_B + I_B) + A_4 (E_H + I_H) + A_5 (E_E + I_E) \\ &\quad + \frac{1}{2} [c_1 u_1^2(T) + c_2 u_2^2(T) + c_3 u_3^2(T)] dt, \end{aligned}$$

where the constants  $A_1, A_2, A_3, A_4, A_5$  are positive weight constants for the state variables,  $c_1, c_2, c_3$  are weight constants or cost balancing factors over time corresponding to each control variable,  $T_F$  is the

terminal or final time, then there exist optimal controls  $[u_1^*(T), u_2^*(T), u_3^*(T)]$  given by

$$\begin{cases} u_1^*(t) = \min \left\{ u_{\max}^1, \max \left[ 0, \frac{(b_L \delta_M N_M + L_M)(1 - L_M/K_M)e_1 \lambda_1}{c_1} \right] \right\}, \\ u_2^*(t) = \min \left\{ u_{\max}^2, \max \left[ 0, \frac{e_2 L_M(1 - L_M/K_M) \lambda_1}{c_2} \right] \right\}, \\ u_3^*(t) = \min \left\{ u_{\max}^3, \max \left[ 0, \frac{e_3 S_M \lambda_2 + e_3 E_M \lambda_3 + e_3 I_M \lambda_4}{c_3} \right] \right\}. \end{cases} \quad (\text{S5})$$

*Proof.* The necessary conditions an optimal control problem must satisfy are defined in the Pontryagin's Maximum Principle (Pontryagin, 2018). The principle converts our optimal control problem together with the objective functional defined in Equation (S5), into a problem of minimizing pointwise the Hamiltonian ( $\mathcal{H}$ ) with respect to the control variables ( $u_1(t), u_2(t), u_3(t)$ ), where the Hamiltonian is given by the formula:

$$\begin{aligned} \mathcal{H} = & A_1 L_M + A_2 N_M + A_3 (E_B + I_B) + A_4 (E_H + I_H) + A_5 (E_E + I_E) \\ & + \frac{1}{2} c_1 u_1^2 + \frac{1}{2} c_2 u_2^2 + \frac{1}{2} c_3 u_3^2 + \lambda_1 L'_M + \lambda_2 S'_M + \lambda_3 E'_M + \lambda_4 I'_M \\ & + \lambda_5 S'_B + \lambda_6 E'_B + \lambda_7 I'_B + \lambda_8 R'_B + \lambda_9 D'_B \\ & + \lambda_{10} S'_H + \lambda_{11} E'_H + \lambda_{12} I'_H + \lambda_{13} R'_H + \lambda_{14} x' + \lambda_{15} D'_H \\ & + \lambda_{16} S'_E + \lambda_{17} V'_E \lambda_{18} E'_E + \lambda_{19} I'_E + \lambda_{20} R'_E + \lambda_{21} D'_E. \end{aligned} \quad (\text{S6})$$

Substituting the derivatives of the state variables, we get:

$$\begin{aligned}
\mathcal{H} = & A_1 L_M + A_2 [S_M + E_M + I_M] + A_3 (E_B + I_B) + A_4 (E_H + I_H) + A_5 (E_E + I_E) \\
& + \frac{1}{2} c_1 u_1^2 + \frac{1}{2} c_2 u_2^2 + \frac{1}{2} c_3 u_3^2 \\
& + \lambda_1 \left[ \{(1 - e_1 u_1) b_L \delta_M (S_M + E_M + I_M) - (\mu_L + e_1 u_1 + e_2 u_2) L_M\} \left[ 1 - \frac{L_M}{K_M} \right] - b_M L_M \right] \\
& + \lambda_2 \left[ b_M L_M - \frac{\delta_M \beta_B I_B S_M}{K_B} - (\mu_M + e_3 u_3) S_M \right] \\
& + \lambda_3 \left[ \frac{\delta_M \beta_B I_B S_M}{K_B} - [\gamma_M + \mu_M + e_3 u_3] E_M \right] \\
& + \lambda_4 [\gamma_M E_M - [\mu_M + e_3 u_3] I_M] \\
& + \lambda_5 \left[ \left[ b_B - (b_B - \mu_B) \frac{N_B}{K_B} \right] N_B - \frac{\delta_M \beta_M \phi_B I_M S_B}{K_M} - \mu_B S_B \right] \\
& + \lambda_6 \left[ \frac{\delta_M \beta_M \phi_B I_M S_B}{K_M} - [\gamma_B + \mu_B] E_B \right] \\
& + \lambda_7 [\gamma_B E_B - [\alpha_B + \mu_B] I_B] \\
& + \lambda_8 [(1 - \nu_B) \alpha_B I_B - \mu_B R_B] \\
& + \lambda_9 [\alpha_B \nu_B I_B] \\
& + \lambda_{10} \left[ b_H N_H - \frac{(1 - x) \delta_M \beta_M \phi_H I_M S_H}{K_M} - \mu_H S_H \right] \\
& + \lambda_{11} \left[ \frac{(1 - x) \delta_M \beta_M \phi_H I_M S_H}{K_M} - [\gamma_H + \mu_H] E_H \right] \\
& + \lambda_{12} [\gamma_H E_H - [\alpha_H + \mu_H] I_H] \\
& + \lambda_{13} [(1 - \nu_H) \alpha_H I_H - \mu_H R_H] \\
& + \lambda_{14} [\kappa x (1 - x) [-1 + \omega I_B]] \\
& + \lambda_{15} [\nu_H \alpha_H I_H] \\
& + \lambda_{16} \left[ b_E N_E - \frac{\delta_M \beta_M \phi_E I_M S_E}{K_M} - (\mu_E + \theta_E) S_E \right] \\
& + \lambda_{17} \left[ \theta_E S_E - (\omega_E + \mu_E) V_E - \frac{(1 - c_E) \delta_M \beta_M \phi_E I_M V_E}{K_M} \right] \\
& + \lambda_{18} \left[ \frac{\delta_M \beta_M \phi_E I_M S_E}{K_M} + \frac{(1 - c_E) \delta_M \beta_M \phi_E I_M V_E}{K_M} - [\gamma_E + \mu_E] E_E \right] \\
& + \lambda_{19} [\gamma_E E_E - [\alpha_E + \mu_E] I_E] \\
& + \lambda_{20} [(1 - \nu_E) \alpha_E I_E - \mu_E R_E] \\
& + \lambda_{21} [\nu_E \alpha_E I_E].
\end{aligned} \tag{S7}$$

The variables  $\lambda_1, \lambda_2, \dots, \lambda_{21}$  are the adjoints to the state variables and should satisfy

$$\begin{aligned}
\lambda'_1 &= -\frac{\partial \mathcal{H}}{\partial L_M}; \lambda'_2 = -\frac{\partial \mathcal{H}}{\partial S_M}; \lambda'_3 = -\frac{\partial \mathcal{H}}{\partial E_M}; \lambda'_4 = -\frac{\partial \mathcal{H}}{\partial I_M}; \lambda'_5 = -\frac{\partial \mathcal{H}}{\partial S_B}; \lambda'_6 = -\frac{\partial \mathcal{H}}{\partial E_B}, \\
\lambda'_7 &= -\frac{\partial \mathcal{H}}{\partial I_B}; \lambda'_8 = -\frac{\partial \mathcal{H}}{\partial R_B}; \lambda'_9 = -\frac{\partial \mathcal{H}}{\partial D_B}; \lambda'_{10} = -\frac{\partial \mathcal{H}}{\partial S_H}; \lambda'_{11} = -\frac{\partial \mathcal{H}}{\partial E_H}; \lambda'_{12} = -\frac{\partial \mathcal{H}}{\partial I_H}; \\
\lambda'_{13} &= -\frac{\partial \mathcal{H}}{\partial R_H}; \lambda'_{14} = -\frac{\partial \mathcal{H}}{\partial x}; \lambda'_{15} = -\frac{\partial \mathcal{H}}{\partial D_H}; \lambda'_{16} = -\frac{\partial \mathcal{H}}{\partial S_E}; \lambda'_{17} = -\frac{\partial \mathcal{H}}{\partial V_E}; \lambda'_{18} = -\frac{\partial \mathcal{H}}{\partial E_E}; \\
\lambda'_{19} &= -\frac{\partial \mathcal{H}}{\partial I_E}; \lambda'_{20} = -\frac{\partial \mathcal{H}}{\partial R_E}; \lambda'_{21} = -\frac{\partial \mathcal{H}}{\partial D_E}.
\end{aligned}$$

Taking partial derivatives, we have

$$\begin{aligned}
\lambda'_1 &= (\mu_L + e_1 u_1 + e_2 u_2) \left[ 1 - \frac{2L_M}{K_M} \right] \lambda_1 + \frac{(1 - e_1 u_1) b_L \delta_M N_M}{K_M} \lambda_1 + (\lambda_1 - \lambda_2) b_M - A_1, \\
\lambda'_2 &= \frac{\delta_M \beta_B I_B}{K_B} [\lambda_2 - \lambda_3] + (\mu_M + e_3 u_3) \lambda_2 - (1 - e_1 u_1) b_L \delta_M \left[ 1 - \frac{L_M}{K_M} \right] \lambda_1 - A_2, \\
\lambda'_3 &= (\gamma_M + \mu_M + e_3 u_3) \lambda_3 - (1 - e_1 u_1) b_L \delta_M \left[ 1 - \frac{L_M}{K_M} \right] \lambda_1 - \gamma_M \lambda_4 - A_2, \\
\lambda'_4 &= \frac{\delta_M \beta_M \phi_B S_B}{K_M} [\lambda_5 - \lambda_6] + \frac{(1 - x) \delta_M \beta_M \phi_H S_H}{K_M} [\lambda_{10} - \lambda_{11}] + (\mu_M + e_3 u_3) \lambda_4 \\
&\quad + \frac{\delta_M \beta_M \phi_E S_E}{K_M} [\lambda_{16} - \lambda_{18}] + \frac{(1 - c_E) \delta_M \beta_M \phi_E V_E}{K_M} [\lambda_{17} - \lambda_{18}] - (1 - e_1 u_1) b_L \delta_M \left[ 1 - \frac{L_M}{K_M} \right] \lambda_1 - A_2, \\
\lambda'_5 &= \frac{\delta_M \beta_M \phi_B I_M}{K_M} [\lambda_5 - \lambda_6] + \mu_B \lambda_5 - \left[ b_B - 2(b_B - \mu_B) \frac{N_B}{K_B} \right] \lambda_5, \\
\lambda'_6 &= (\gamma_B + \mu_B) \lambda_6 - \gamma_B \lambda_7 - \left[ b_B - 2(b_B - \mu_B) \frac{N_B}{K_B} \right] \lambda_5 - A_3, \\
\lambda'_7 &= \frac{\delta_M \beta_M S_M}{K_B} [\lambda_2 - \lambda_3] + (\alpha_B + \mu_B) \lambda_7 - (1 - \nu_B) \alpha_B \lambda_8 - \alpha_B \nu_B \lambda_9 \\
&\quad - \left[ b_B - 2(b_B - \mu_B) \frac{N_B}{K_B} \right] \lambda_5 - \kappa x (1 - x) \omega \lambda_{14} - A_3, \\
\lambda'_8 &= \mu_B \lambda_8 - \left[ b_B - 2(b_B - \mu_B) \frac{N_B}{K_B} \right] \lambda_5, \\
\lambda'_9 &= 0 \\
\lambda'_{10} &= \frac{(1 - x) \delta_M \beta_M \phi_H I_M}{K_M} [\lambda_{10} - \lambda_{11}] + \mu_H \lambda_{10} - b_H \lambda_{10}, \\
\lambda'_{11} &= (\gamma_H + \mu_H) \lambda_{11} - \gamma_H \lambda_{12} - b_H \lambda_{10} - A_4, \\
\lambda'_{12} &= (\alpha_H + \mu_H) \lambda_{12} - (1 - \nu_H) \alpha_H \lambda_{13} - \nu_H \alpha_H \lambda_{15} - b_H \lambda_{10} - A_4, \\
\lambda'_{13} &= \mu_H \lambda_{13} - b_H \lambda_{10}, \\
\lambda'_{14} &= \frac{\delta_M \beta_M \phi_H I_M S_H}{K_M} (\lambda_{11} - \lambda_{10}) - \kappa (1 - 2x) (\omega I_B - 1) \lambda_{14}, \\
\lambda'_{15} &= 0, \\
\lambda'_{16} &= \frac{\delta_M \beta_M \phi_E I_M}{K_M} [\lambda_{16} - \lambda_{18}] + \theta_E [\lambda_{16} - \lambda_{17}] + (\mu_E - b_E) \lambda_{16}, \\
\lambda'_{17} &= (\omega_E + \mu_E) \lambda_{17} + \frac{(1 - c_E) \delta_M \beta_M \phi_E I_M}{K_M} (\lambda_{17} - \lambda_{18}) - b_E \lambda_{16}, \\
\lambda'_{18} &= (\gamma_E + \mu_E) \lambda_{18} - \gamma_E \lambda_{19} - b_E \lambda_{16} - A_5, \\
\lambda'_{19} &= (\alpha_E + \mu_E) \lambda_{19} - (1 - \nu_E) \alpha_E \lambda_{20} - \nu_E \alpha_E \lambda_{20} - b_E \lambda_{16} - A_5, \\
\lambda'_{20} &= \mu_E \lambda_{20} - b_E \lambda_{16}, \\
\lambda'_{21} &= 0,
\end{aligned} \tag{S8}$$

with transversality conditions  $\lambda_1(T) = \lambda_2(T) \cdots = \lambda_{21}(T) = 0$ . Moreover,  $[u_1^*(t), u_2^*(t), u_3^*(t)]$  satisfy the conditions

$$\frac{\partial \mathcal{H}}{\partial u_1} = 0, \quad \frac{\partial \mathcal{H}}{\partial u_2} = 0, \quad \frac{\partial \mathcal{H}}{\partial u_3} = 0,$$

implying that;

$$\begin{cases} c_1 u_1 - e_1 b_L \delta_M N_M \left[ 1 - \frac{L_M}{K_M} \right] \lambda_1 - e_1 L_M \left[ 1 - \frac{L_M}{K_M} \right] \lambda_1 = 0, \\ c_2 u_2 - e_2 L_M \left[ 1 - \frac{L_M}{K_M} \right] \lambda_1 = 0, \\ c_3 u_3 - e_3 \lambda_2 S_M - e_3 \lambda_3 E_M - e_3 \lambda_4 I_M = 0, \end{cases} \quad (\text{S9})$$

in the interior of the control set  $\mathcal{U}$ . Solving Equation (S9) for  $(u_1, u_2, u_3)$  in  $\mathcal{U}$ , we get the optimal solution as:

$$\begin{cases} u_1^*(t) = \min \left\{ u_{\max}^1, \max \left[ 0, \frac{(b_L \delta_M N_M + L_M)(1 - L_M/K_M)e_1 \lambda_1}{c_1} \right] \right\}, \\ u_2^*(t) = \min \left\{ u_{\max}^2, \max \left[ 0, \frac{e_2 L_M (1 - L_M/K_M) \lambda_1}{c_2} \right] \right\}, \\ u_3^*(t) = \min \left\{ u_{\max}^3, \max \left[ 0, \frac{e_3 S_M \lambda_2 + e_3 E_M \lambda_3 + e_3 I_M \lambda_4}{c_3} \right] \right\}. \end{cases} \quad (\text{S10})$$

The values of  $\lambda_i$ , for  $i = 1, \dots, 21$  are obtained by solving system (S8). □

## S2.1 Scenario 1: Use of mosquito reduction methods $u_1$ , $u_2$ , $u_3$

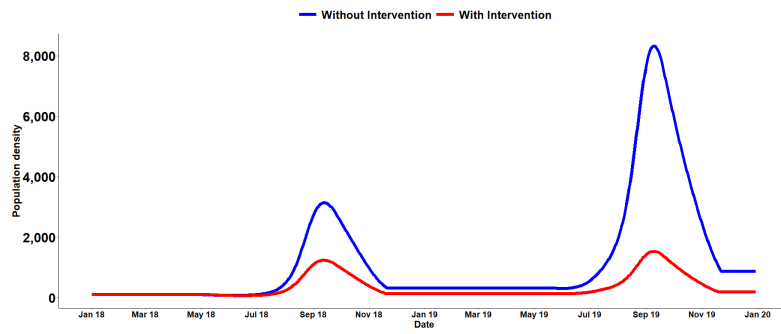

(a) WNV infectious mosquitoes.

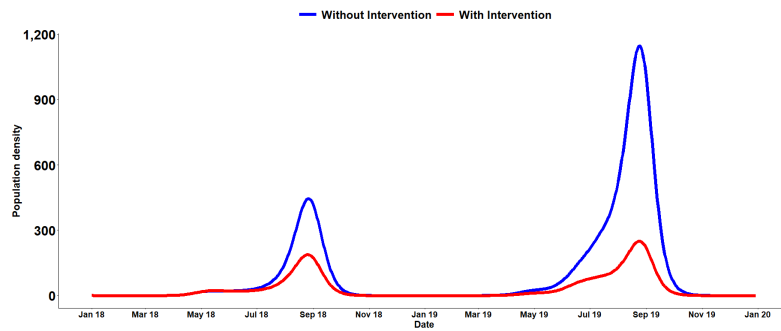

(b) WNV infectious birds.

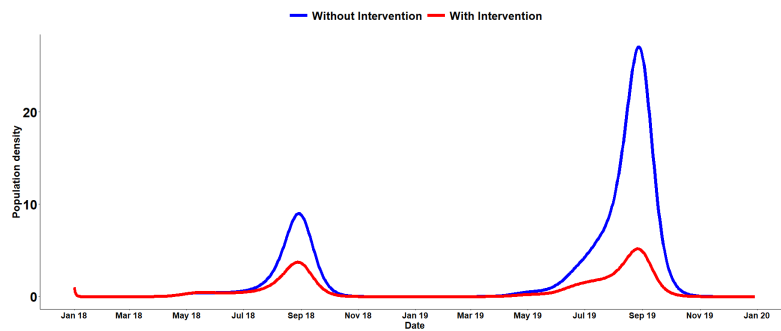

(c) WNV infected humans.

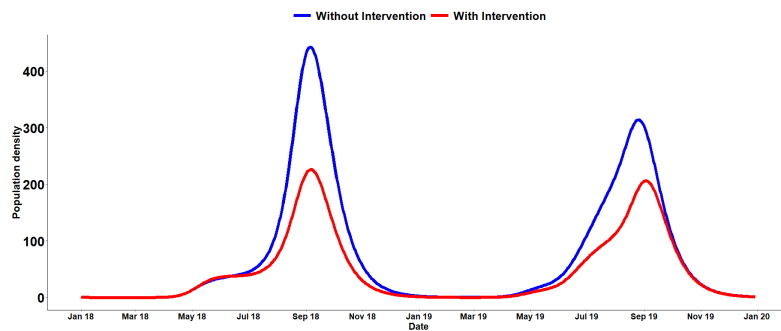

(d) WNV infected equids.

Figure S1: Impact of using mosquito control methods: the physical removal and destruction of potential mosquito breeding sites ( $u_1$ ), the use of larvicides ( $u_2$ ) and the use of adulticides ( $u_3$ ), i.e. Scenario 1.

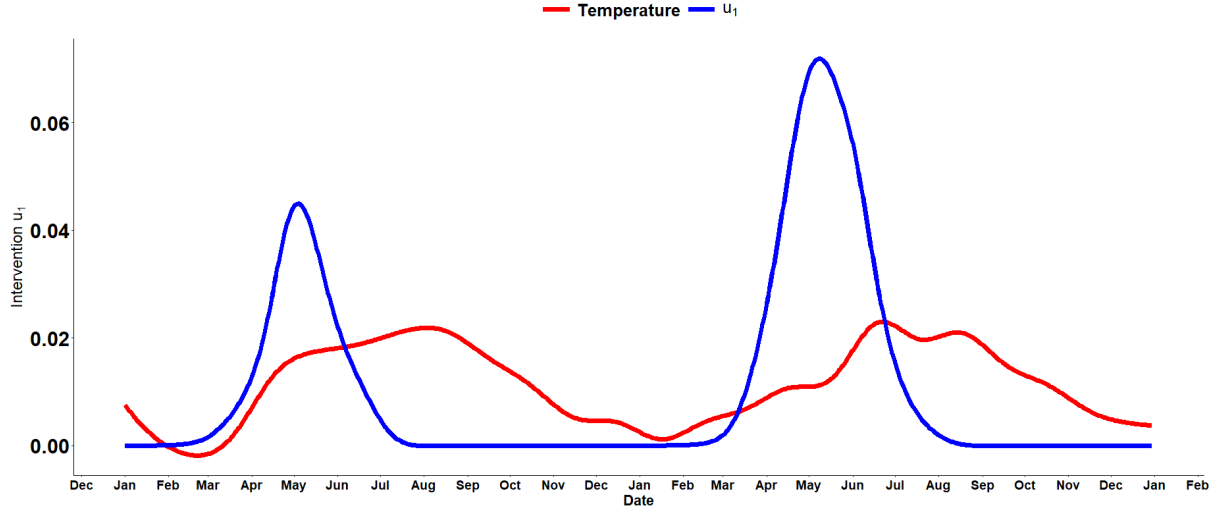

(a) Physical removal and destruction of potential mosquito breeding sites ( $u_1$ ).

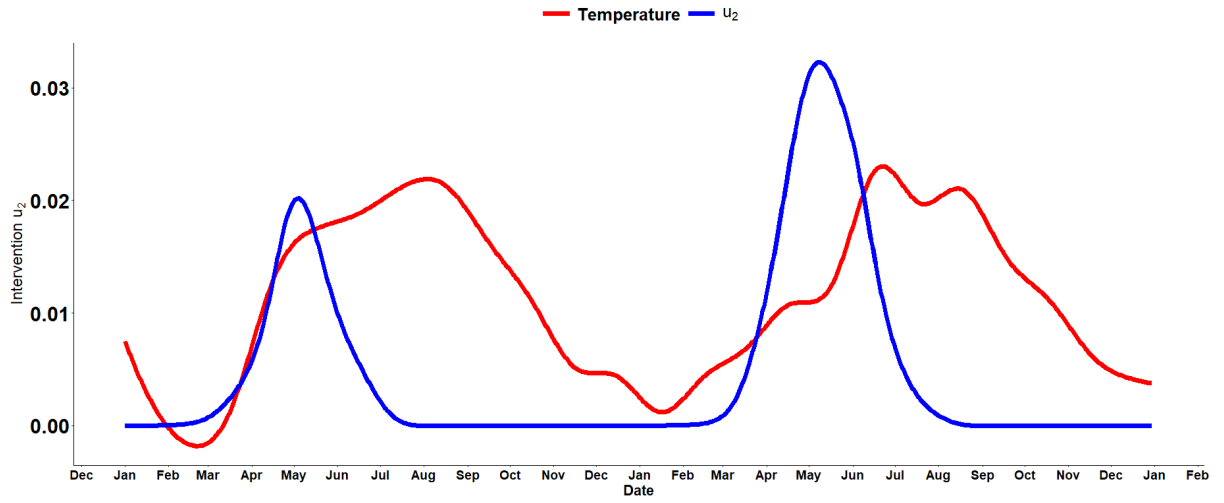

(b) Use of larvicides ( $u_2$ ).

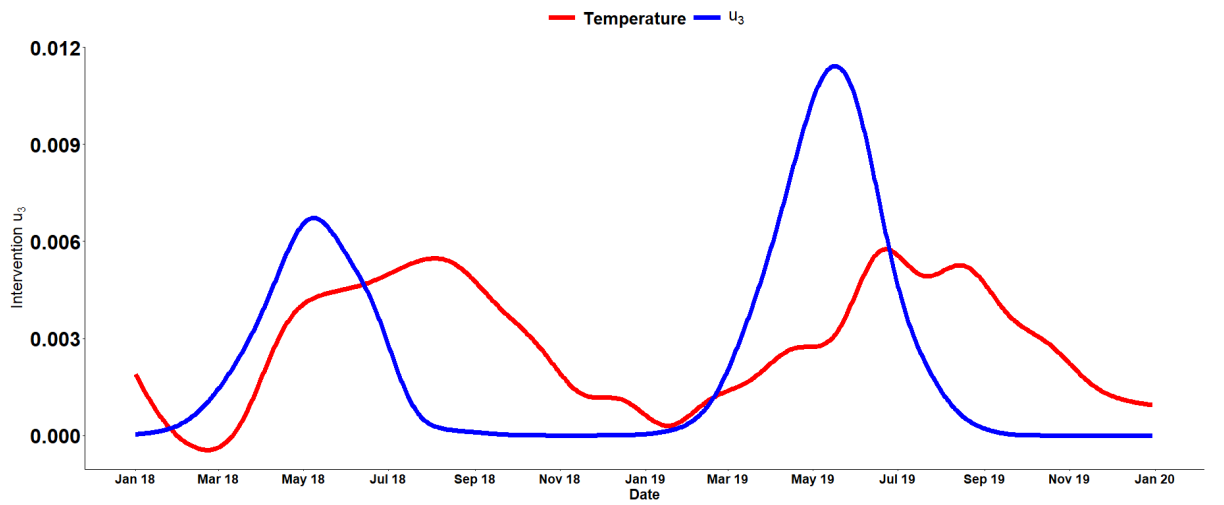

(c) Use of adulticides ( $u_3$ ).

Figure S2: Control profiles showing when mosquito control methods can be initiated, with  $e_1 = e_2 = e_3 = 0.9, A_1 = A_2 = A_3 = 1 \times 10^{-9}, A_4 = 1.0, A_5 = 0.1, c_1 = c_2 = 1, c_3 = 10^6$ .

## References

- Vincent Laperriere, Katharina Brugger, and Franz Rubel. Simulation of the seasonal cycles of bird, equine and human west nile virus cases. *Preventive Veterinary Medicine*, 98(2–3):99–110, February 2011. ISSN 0167-5877. doi: 10.1016/j.prevetmed.2010.10.013. URL <http://dx.doi.org/10.1016/j.prevetmed.2010.10.013>.
- L.S. Pontryagin. *Mathematical Theory of Optimal Processes*. Routledge, May 2018. ISBN 9780203749319. doi: 10.1201/9780203749319. URL <http://dx.doi.org/10.1201/9780203749319>.
- P van den Driessche and James Watmough. Reproduction numbers and sub-threshold endemic equilibria for compartmental models of disease transmission. *Mathematical Biosciences*, 180(1–2): 29–48, November 2002. ISSN 0025-5564. doi: 10.1016/s0025-5564(02)00108-6. URL [http://dx.doi.org/10.1016/s0025-5564\(02\)00108-6](http://dx.doi.org/10.1016/s0025-5564(02)00108-6).
